# Supplementary material for: An Inexact Semi-smooth Newton Method on Riemannian Manifolds with Application to Duality-based Total Variation Denoising
Source: arXiv:2102.10309 source file (2021-08-16)
Supplement: Supplementary file 1 [file A-Appendix.tex]

- The explicit forms for the proxes and derivatives are useful but should go into an appendix
