# Supplementary material for: An Inexact Semi-smooth Newton Method on Riemannian Manifolds with Application to Duality-based Total Variation Denoising
Source: arXiv:2102.10309 source file (2021-08-16)
Supplement: Supplementary file 2 [file main.tex]

\documentclass{article}
\usepackage[utf8]{inputenc}
\usepackage{lipsum}
\usepackage{amsfonts}
\usepackage{graphicx}
\usepackage{epstopdf}
\usepackage{algorithmic}
\usepackage{enumerate}
\usepackage{csquotes}
\usepackage{todonotes}
%\usepackage[inline]{asymptote}
\usepackage{subcaption}
\usepackage{wrapfig}

\title{Results PD-RSSN}
\author{wd292 }
\date{May 2021}

\begin{document}

\maketitle

\section{Convergence Behaviour of PD-RSSN for Different Problem Sizes}
In this experiment

Main points will be
\begin{itemize}
	\item in this experiment we will look at the amount of steps needed to converge for different problem sizes
	\item this is important since doing a Newton step will scale quadratically at best (only when we accelerate right)?
	\item So we need the method not to scale poorly with respect to problem size
	\item Even though, this is in general hard to measure fairly, because the problem will be different at different scales. 
	\item In order to get some intuition we will repeat the experiment described in previous section, but with different scales. (do we also want lRCPA here? it is a bit hard to see what happens to the steps for RSSN)
	\item Bewcause of the wide range of iteratoins needed for lRCPA to converge, we focus on RSSN here
	\item For S2 we will use 10, 15, 20, 25 and 30
	\item For SPD3 we will use 4, 7, 10, 13 and 16
	\item We observe the behavriour we hope for
\end{itemize}

\begin{figure}[h!]
	\includegraphics[width=0.45\linewidth]{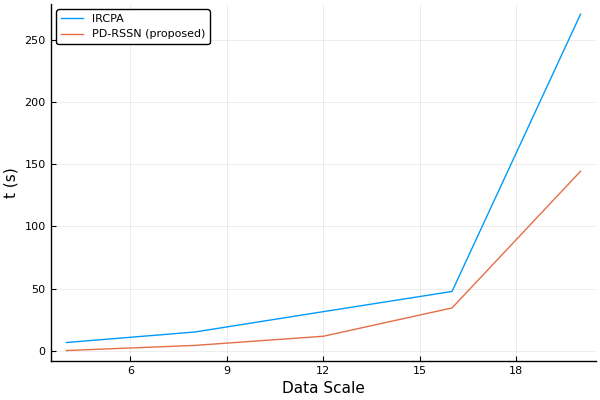}
	\includegraphics[width=0.45\linewidth]{experiments/article-RSSN-scaling-of-algorithm-2021-05-06-11-49-03/timing-S2.png}
\end{figure}

\begin{figure}[h!]
	\includegraphics[width=0.45\linewidth]{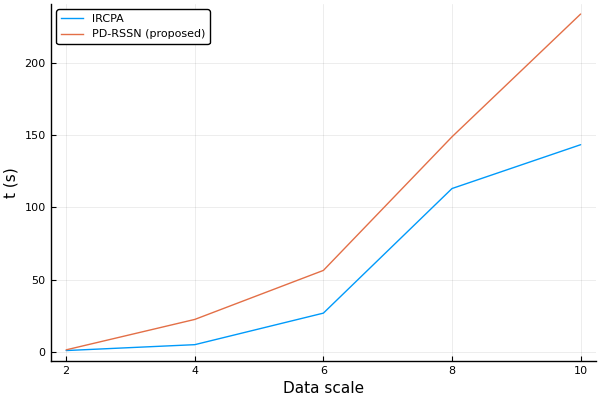}
	\includegraphics[width=0.45\linewidth]{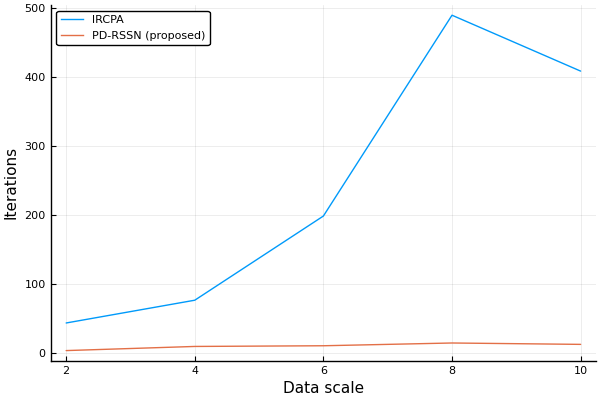}
\end{figure}


\end{document}
